# Supplementary material for: A conveyor-belt magneto-optical trap of CaF
Source: arXiv:2409.15262 source file (2024-09-24)
Supplement: Supplementary file 1 [file supplmat.tex]

\documentclass[aps,amsmath,amssymb,prl,superscriptaddress]{revtex4}  % for PRL

\usepackage{graphicx}
\usepackage{epstopdf}
\usepackage{color}
\definecolor{orange}{RGB}{255,127,0}
\definecolor{blue2}{RGB}{33,114,173}
\usepackage{bm}% bold math
\usepackage{soul}
\usepackage{braket,gensymb,tikz}
\usepackage{float}
\usepackage{graphicx}% Include figure files
\usepackage{xcolor} %textcolor
\usepackage{hyperref}
\begin{document}

\title{Supplemental Material for ``A conveyor-belt magneto-optical trap of CaF'}

\author{Scarlett S. Yu}
\author{Jiaqi You}
\author{Yicheng Bao}
\altaffiliation[Current address: ]{Department of Physics, Princeton University, Princeton, NJ 08544, USA}
\affiliation{Department of Physics, Harvard University, Cambridge, MA 02138, USA}
\affiliation{Harvard-MIT Center for Ultracold Atoms, Cambridge, MA 02138, USA}

\author{Lo\"ic Anderegg}
\altaffiliation[Current address: ]{Department of Physics and Astronomy, University of Southern California, Los Angeles, CA 90089, USA}
\affiliation{Department of Physics, Harvard University, Cambridge, MA 02138, USA}
\affiliation{Harvard-MIT Center for Ultracold Atoms, Cambridge, MA 02138, USA}

\author{Christian Hallas}
\author{Grace K. Li}
\affiliation{Department of Physics, Harvard University, Cambridge, MA 02138, USA}
\affiliation{Harvard-MIT Center for Ultracold Atoms, Cambridge, MA 02138, USA}

\author{Dongkyu Lim}
\author{Eunmi Chae}
\affiliation{Department of Physics, Korea University, Seongbuk-gu, Seoul 02841, South Korea}

\author{Wolfgang Ketterle}
\affiliation{Harvard-MIT Center for Ultracold Atoms, Cambridge, MA 02138, USA}
\affiliation{Department of Physics, Massachusetts Institute of Technology, Cambridge, MA 02139, USA}

\author{Kang-Kuen Ni} 
\affiliation{Department of Physics, Harvard University, Cambridge, MA 02138, USA}
\affiliation{Harvard-MIT Center for Ultracold Atoms, Cambridge, MA 02138, USA}
\affiliation{Department of Chemistry and Chemical Biology, Harvard University, Cambridge, MA 02138, USA}

\author{John M. Doyle} 
\affiliation{Department of Physics, Harvard University, Cambridge, MA 02138, USA}
\affiliation{Harvard-MIT Center for Ultracold Atoms, Cambridge, MA 02138, USA}

\maketitle

\makeatletter
\renewcommand \thesection{S\@arabic\c@section}
\renewcommand\thetable{S\@arabic\c@table}
\renewcommand \thefigure{S\@arabic\c@figure}
\makeatother

\section{Experimental sequence details}  \label{sequence}

%CaF molecules first chemically produced from laser ablated calcium atoms and sulfur hexafluoride (SF6) gas in a cryogenic buffer-gas cell.
The experiment proceeds through four general stages: (1) RF MOT, (2) Sub-Doppler cooling, (3) Conveyor MOT, and (4) ODT loading. 
\begin{enumerate}
\renewcommand\labelenumi{(\theenumi)}
    \item  RF MOT: CaF molecules are initially captured in a radio-frequency (RF) red-detuned MOT operating on $X(\nu =0, N=1)  - A(\nu' =0, J'=1/2)$ cooling transition at 606~nm, as described in \cite{anderegg2017radio, bao2022fast}. Three pairs of orthogonal beams, each containing the frequency components addressing the four ground-state hyperfine states in the $N=1$ rotational manifold, are sent into the center of the MOT chamber and retro-reflected using a quarter-wave plate and a mirror. The frequency sidebands are generated by a set of acousto-optic modulators, allowing for independent control of polarization and intensity for each hyperfine component.   
    A Pockels cell enables rapid polarization switching. To maximize the number of trapped molecules while minimizing the heating, we begin with magnetic field gradient of $\sim$ 20~G/cm and a full beam intensity of $I_o = 300$~mW/cm$^2$ ($\sim 6 I_\text{sat}$) at a detuning of $\Delta = -8$~MHz to  for 5~ms load the MOT. The intensity is then lowered to $I_o/4$ over 5~ms to allow for thermalization at lower temperature, while magnetic field gradient is ramped to $\sim$ 50~G/cm RMS, compressing the molecular cloud to $\lesssim 600~\mu$m. A 1-ms resonant light pulse is used to image the molecules, which is then converted to a molecular number following a calibration procedure described in the appendix of our previous work~\cite{bao2022fast}. % up to $2 \times 10^5$ trapped molecules are observed.
\item Sub-Doppler and $\Lambda$ cooling: In the next 5~ms, we turn off the RF field and Pockels cell, jumping the laser intensity and detuning first to the sub-Doppler cooling parameters \cite{anderegg2018laser} with $\Delta = +34$ MHz. %Sub-Doppler cooling provides larger trapping forces and higher base tempeature. 
This is followed by a 5-ms $\Lambda$-cooling pulse, which reduces the cloud temperature to a base temperature of 18(5)~$\mu$K while retaining $\sim 80\%$ of the loaded molecules. 

\item Conveyor MOT compression: To load the molecules into a DC conveyor MOT, we switch MOT light frequency to the scheme shown in Fig.~1(b) of main text and the magnetic field from RF to DC configuration.  After 30 ms, the cloud compresses to 64(5)~$\mu$m. To measure its spatial profile of the conveyor MOT cloud, we hold the magnetic field for an additional 10 ms to collect the in-situ fluorescence signal.
%$S_\text{conveyor}$. For normalization (e.g. to remove fluctuations in molecular flux from the cryogenic buffer gas source), $S_\text{conveyor}$ is referenced against $S_\text{red}$, to remove fluctuations in the molecular flux from the cryogenic buffer gas source.

\item ODT loading: After switching off all MOT light and the DC magnetic field, we turn on the 1064 nm trap light with $\Lambda$-cooling applied for 3~ms. After holding the molecules in ODT for 100~ms to ensure the background cloud has fully dissipated, a 1-ms resonant pulse is used to collect the ODT signal. To obtain stable ODT loading efficiency measurements, for each experimental cycle, we use a 5-ms in-situ fluorescence collected at the end of the conveyor MOT compression as a refernece signal to remove fluctuations in the molecular flux from the cryogenic buffer gas source. 
\end{enumerate}

For further details such as molecular beam preparation, see our previous publications \cite{anderegg2017radio, bao2022fast}.

\section{RF - DC MOT coil switching}

Transitioning the magnetic field from RF to DC MOT configuration presents several technical challenges as it requires isolating the RF and DC parts of the MOT coils’ tank circuit while maintaining RF resonance. We address this by employing high-impedance inductors and back-to-back solid-state relays.

Isolation is critical here because the high voltages in the RF MOT can couple into the DC current supply ground, causing interference and instability; proper isolation ensures the integrity of both the RF and DC systems. Our MOT coils consist of a pair of in-vacuum magnetic coils, forming a resonant tank circuit along with variable capacitors. Each tank circuit is independently driven by a custom-built 1~kW RF amplifier operating at 1 MHz. This setup generates a magnetic field gradient of up to 50~G/cm RMS during the MOT compression, corresponding to peak-to-peak voltages of $\sim 4$~kV. While mechanical relays are capable of handling high voltages, they have limited lifetimes and slower switching times. In contrast, solid-state relays offer longer lifetimes and faster switching but are limited by their lower working voltage range. To overcome this, we use homemade high-impedance inductors ($Z_L = 10,668~\Omega$) to isolate the RF from the DC circuit. The DC current is applied to a capacitor with $Z_C \simeq 1 ~\Omega$ with self-resonance frequency greater than 1 MHz, and connected to the MOT coil through the high-impedance inductor. To reduce switching time, a damping resistor is placed in parallel with $Z_C$. This setup significantly reduces the voltage across the relay by a factor of 10,000, ensuring efficient switching and reliable operation during the transition from RF to DC operation.

\section{Conveyor MOT lifetime and scattering rate }
To measure the lifetime of the conveyor MOT, after the compression stage, we hold the the magnetic field at 40~G/cm for variable amount time while monitoring the remaining molecules. Figure \ref{fig:MOT_lifetime} shows the decay in fluorescence signal (or the number of trapped particles) as a function of hold time. The result fits to a single exponential decay with a fitted lifetime $\tau_\text{conveyor} = $ 37(8)~ms, consistent with the absence of light-assisted two-body collisions at this density.
\begin{figure}[!h]
  \centering
  \includegraphics[width=0.5\textwidth]{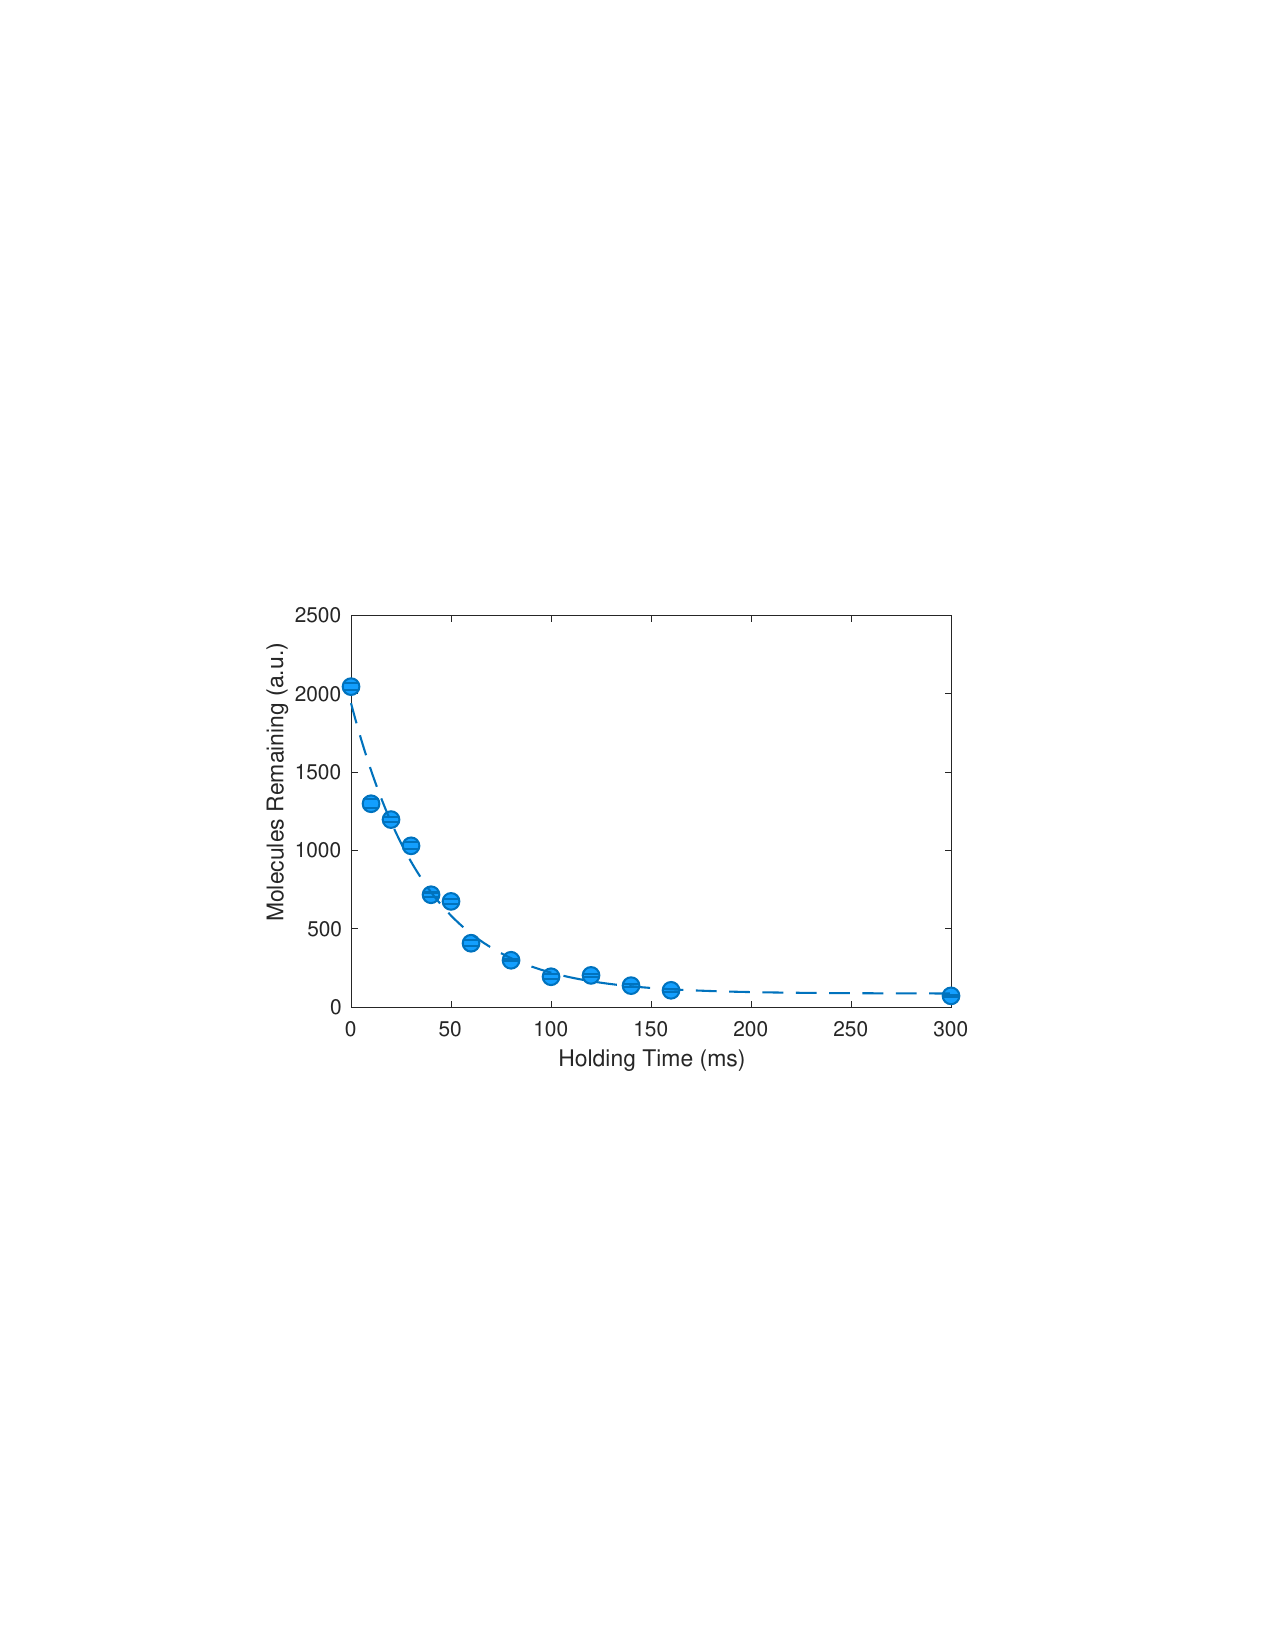}
  \caption{Number of remaining trapped molecules in the conveyor MOT as a function of holding time, with the magnetic field gradient set at 40 G/cm. The fitted lifetime is $\tau_\text{conveyor} = $ 37(8)~ms. }
  \label{fig:MOT_lifetime}
\end{figure}

 When molecules are exposed to the light and scatter photons for a given time, they have a certain probability to decay to unaddressed vibrational state(s). By turning off selective repumping lasers and holding the molecules in the conveyor MOT for variable time, we allow the population to accumulate in unaddressed states, effectively limiting the number of photons that can be scattered. The scattering rate is then extracted from the observed lifetime and known vibrational branching ratios.
 
 During the holding period, decay in molecular signal can occur due to various mechanisms, such as optical pumping into unaddressed vibrational states or trap loss. To isolate the loss due to finite photon budget, we fix the total holding time at 40~ms and vary the duration $T_\text{off}$ during which $v=2$ and $v=3$ vibrational repumps are turned off. %This way, we can specifically probe the loss due to limited photons. 
 This reduces the photon budget per molecule from $N_{\text{photon}}$ = $9 \times 10^5$ to $1350$. Figure \ref{fig:MOT_scatt} shows the fluorescence decay as a function of $T_\text{off}$. An exponential fit in th where $v=2$ and $v=3$ repumps are off yields a lifetime of $\tau_\text{reduced} = 4.9(0.6)$~ms, and the corresponding scattering rate is calculated to be $\Gamma= N_{\text{photon}} /\tau_{\text{reduced}} =$ $0.27(3) \times 10^6 \text{ s}^{-1}$. %Since other loss mechanisms remain unaffected during the fixed holding time, the scattering rate $\gamma$ can be calculated using $\gamma = N_{\text{photon}} /\tau_{\text{off}}$, where $N_{\text{photon}}$ is the reduced photon budget. Substituting the values, we find the scattering rate of the conveyor MOT at 40 G/cm to be $\gamma = 276$ kHz.
\begin{figure}[!ht]
  \centering
  \includegraphics[width=0.5\textwidth]{Scattering Rate measurement.pdf}
  \caption{Number of remaining molecules as a function of $T_\text{hold}$ during which  $v=2$ and $v=3$ repumping lasers are turned off. The data has an exponential decay with a fitted lifetime $\tau_{\text{reduced}} = 4.9(0.6)$~ms due to finite photon budget.}
  \label{fig:MOT_scatt}
\end{figure}

\section{Temperature measurements}
We use a standard time-of-flight expansion method to determine the temperature of a thermal molecular cloud, assuming a Gaussian density distribution in the conveyor MOT or ODT. By turning off all the trap light and magnetic field, we allow the the molecular cloud to freely expand for variable length of time $t_\text{TOF}$ and use a subsequent $1$-ms resonant light pulse for imaging. As resonant imaging on the molecular can cause heating, and consequently, extra expansion, the 1~ms exposure time is chosen here as it is short compared to the expansion time and causes negligible heating. We verified that the size measurements with a 1~ms exposure were similar with those using a shorter 0.5 ms exposure. We fit the molecular image along the radial (axial) direction to a 1D Gaussian to obtain the cloud radius in radial (axial) direction, $\sigma_\text{rad}$ ($\sigma_{ax}$), and extract the corresponding radial (axial) temperature $T_\text{rad}$ ($T_\text{ax}$) from the fitted slope.
The final temperature reported is the geometric mean of radial and axial temperatures: $T= T^{2/3}_{\text{rad}} T^{1/3}_{\text{ax}}$.

\section{ODT loading dynamics and losses}
To better understand the dominant loss mechanisms during the loading process, we examine the time dependence of the ODT loading. From the loading curves in Figure 4(b), We find that the loading dynamics is well captured by four parameters: a loading rate $R(t)$ which depends on the reservoir cloud and its overlap with the ODT, a one-body decay rate $\Gamma$ due to collisions with background gas in the chamber, and a two-body collision rate $\beta'$ caused by light-assisted collision \cite{Schlosser:2001prv, schlosser2002ODT_LAC}. They follow a rate equation model commonly used for atoms \cite{heazlewood2021towards}. 
\begin{equation} \label{ODT_eq}
   \frac{dN(t)}{dt} = R(t) - \Gamma N -\beta'  N^2
\end{equation}
%where $R(t)$ is the loading rate, which depends on the dynamics in the reservoir cloud and its spatial overlap with the ODT, $\Gamma$ is the one-body loss rate due to photon scattering from the $\Lambda$-cooling light and vacuum lifetime, and $\beta'$ is the two-body loss rate caused by light-assisted collisions \cite{Schlosser:2001prv, schlosser2002ODT_LAC}. 
$R(t)=R_o e^{-\gamma t}$ sets the initial increase in the loading and accounts for the total decay rate $\gamma$ in the cloud reservoir arising from two processes: (1) the loss of molecules due to cloud expansion out of the ODT trapping volume, and (2) the depletion of molecules as they are successfully loaded into the ODT. %The lower bound of the loss rate $\gamma_L$ can be estimated by experimentally measuring the loss rate contribution from the first process. %By observing the expansion of the reservoir cloud in the presence of $\Lambda$-cooling light for variable amount of time, we find the fluorescence signal follows an exponential decay $R(t) = R_o e^{-\gamma t}$ with a $\gamma_\text{L} = 0.87 \pm 0.44 \text{ ms}^{-1}$.
To determine whether two-body collisional loss plays a role in limiting the loading, we measure the lifetime of molecules $\tau$ in the ODT in presence of $\Lambda$-light. We first load the ODT with $\Lambda$-cooling light under optimal condition and wait for $100$~ms to ensure the background cloud has fully dissipated. Then, we hold the molecules in trap for $260$~ms and apply $\Lambda$-cooling for a variable length of time to induce light-assisted collisions~\cite{cheuk2020observation, anderegg2021observation}. Fitting the data including the two-body loss term yields a $\tau$  that is statistically indistinguishable from that obtained using a single-body loss model (Fig.~4(c)), thus the two-body $\beta^{'}$ term does not dominate over $\Gamma$ under the experimental conditions, indicating that two-body loss does not significantly contribute in this system.
We fit the numerical solution of Eq.~(1) to each loading curve in Fig.~4(b), using the same cloud reservoir decay rate $\gamma$ for all curves, and a fixed one-body rate constant $\Gamma$ extracted from Fig.~4(c) measurement. The free parameters are $\gamma$ and $R_o$. %The free parameters are $\gamma$, with a lower-bound set by $\gamma_\text{L}$, and $R_o$.
% For each loading curve in Fig 4(b), the extracted rate constant $\Gamma$ 
% The extracted rate constants $\gamma$ and $\Gamma$ are fixed in the fitting of the numerical solution of each loading curve in Fig.\ref{fig:4} (b).
\section{ODT alignment}
We examined how the spatial overlap between the ODT and conveyor MOT affects the loading efficiency. We vary the ODT position while monitoring the molecular signal in the ODT. The data are fitted to a Gaussian distribution with $\sigma_{\text{loading}} = 111(12)~\mu$m, which is comparable to the cloud size after 1 ms of diffusive expansion,\ as shown in Fig.~\ref{fig:ODTpos}.  These results are consistent with the rapid loading timescale and indicate that optimizing the spatial overlap between the MOT and ODT is crucial for enhancing loading efficiency.
\begin{figure}[!hb]
  \centering
  \includegraphics[width=0.6\textwidth]{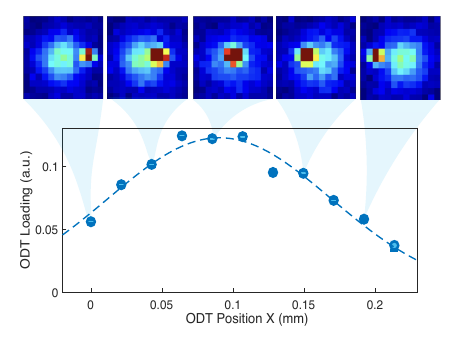}
  \caption{ODT loading efficiency versus ODT position. The loading efficiency is plotted against the center position of the ODT, and the data are fitted to a Gaussian distribution with a width of $\sigma_{\text{loading}} = 111(12)$~\textmu m.}
  \label{fig:ODTpos}
\end{figure}

\section{Effect of ODT trap depth}
\begin{figure}[!hb]
  \centering
  \includegraphics[width=0.5\textwidth]{ODT Lading vs. ODT Intensity v2.pdf}
  \caption{ODT loading efficiency versus ODT powers. The loading efficiency increases with higher ODT light intensities, indicating potential for further improvement by increasing the trap depth and volume.}
\label{fig:ODTintensity}
  \label{fig:ODTintensity}
\end{figure}
We investigate the effect of trap depth by measuring the loading efficiency at various ODT intensities. As shown in Fig.~\ref{fig:ODTintensity}, the loading efficiency increases with intensity, suggesting further improvements are possible with a higher trap depth, though this is currently constrained by technical limitations.

 %The calibration process for determining the absolute molecule number follows the method described in reference [Fast optical transport]. 

\bibliography{caf_bmot.bib}

\end{document}
